# Supplementary material for: Magnetoconductance evolution across the topological-trivial phase transition in ${In_{x}}({Bi_{0.3}}{Sb_{0.7}})_{2-x}{Te_3}$ thin films
Source: arXiv:2512.15185 ancillary file (2025-12-17)
Supplement: Supplementary file 1 [file supplimentary.pdf]

# Supplemental material for "Magnetoconductance evolution across the topological–trivial phase transition in $In_x(Bi_{0.3}Sb_{0.7})_{2-x}Te_3$ thin films"

Sambhu G Nath, Subhadip Manna, Kanav Sharma, Amar Verma, Ritam Banerjee, R K Gopal, Chiranjib Mitra

Indian Institute of Science Education and Research Kolkata, Mohanpur 741246, West Bengal, India

## 1: Thin films characterization.

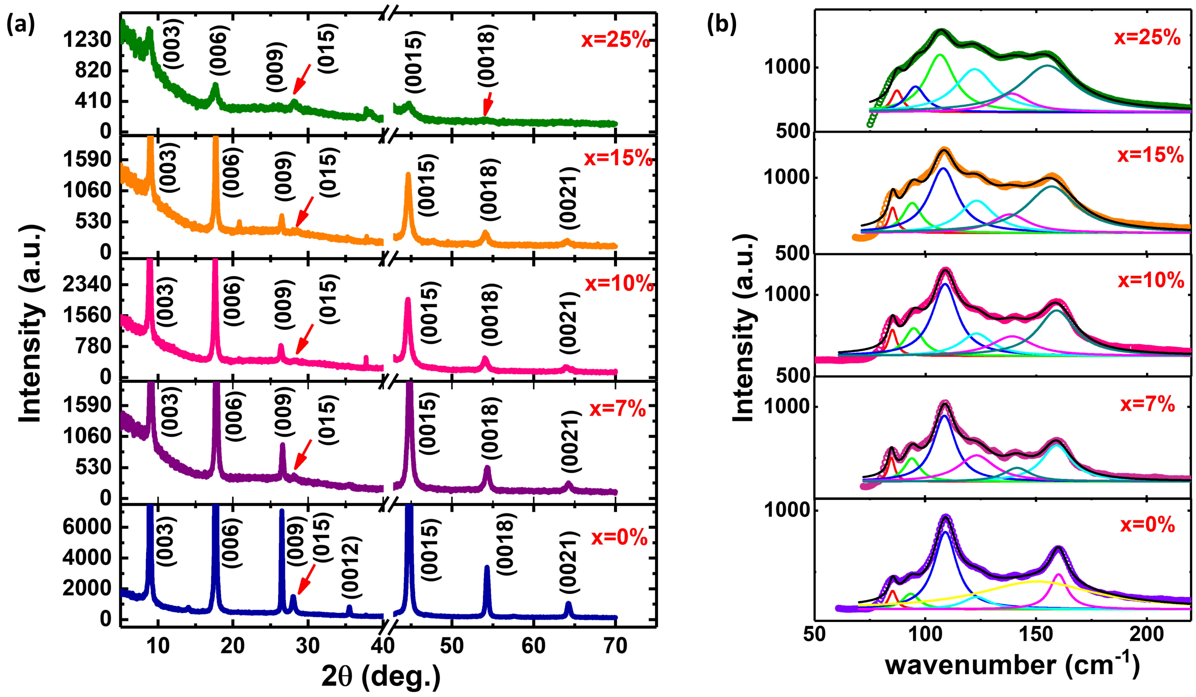


Figure 1: [a] XRD patterns of $In_x(Bi_{0.3}Sb_{0.7})_{2-x}Te_3$ thin films for different indium concentration $x$. [b] Micro-Raman spectra of the corresponding films, showing the evolution of vibrational modes with varying $x$. Individual phonon features have been extracted through multi-Lorentzian deconvolution.

Structural characterization of the PLD-grown $In_x(Bi_{0.3}Sb_{0.7})_{2-x}Te_3$ samples was performed using X-ray diffraction (XRD), micro-Raman spectroscopy with a 532 nm excitation wavelength, and scanning electron microscopy (SEM). XRD measurements provide clear insight into how indium incorporation alters the structural quality of the $In_x(Bi_{0.3}Sb_{0.7})_{2-x}Te_3$ films. In the undoped sample ($x = 0$), the diffraction pattern displays sharp and well-defined $(003n)$ reflections, characteristic of highly oriented $c$-axis growth [16].

Upon introducing indium, a systematic reduction in diffraction peak intensity is observed. For $x = 7\%$, the $(003n)$ peaks remain visible with linewidths similar to the undoped film, though their reduced intensities signal the onset of compositional disorder. As the In concentration increases, peak intensities continue to weaken due to increased lattice distortions and the disruption of long-range structural coherence. In particular, in the intermediate doping regime ($7\% \leq x \leq 15\%$), the $c$-axis lattice parameter remains nearly constant at approximately 27 Å, suggesting that the out-of-plane spacing is relatively insensitive to moderate In substitution, even as the disorder grows [25].

At higher dopings, such as $x = 25\%$, the diffraction pattern exhibits extremely weak or missing peaks. This behavior reflects a transition toward a highly disordered or partially amorphous structure, where indium-induced lattice distortions become sufficiently strong to suppress periodicity over large length scales. Consequently, the XRD signal no longer displays well-resolved Bragg reflections, marking a substantial degradation of the crystalline order at high indium concentrations.

The micro-Raman spectrum of the undoped $In_0(Bi_{0.3}Sb_{0.7})_2Te_3$ film exhibits three well-defined

vibrational features that are characteristic of layered quintuple-layer structures. The $E_g^2$ mode at approximately 109.22 $cm^{-1}$ corresponds to in-plane vibrations involving the Bi/Sb and Te atoms within the quintuple layers. In contrast, the out-of-plane vibrational modes $A_{1g}^1$ and $A_{1g}^2$ appear near 84.97 $cm^{-1}$ and 160 $cm^{-1}$, respectively [25]. In addition to these Raman-allowed modes, weak signatures of the IR-active $A_{1u}^1$ and $A_{1u}^2$ modes are also [21]. Their presence is commonly attributed to finite-size effects, structural imperfections, and symmetry relaxation in thin films, which weaken the strict Raman selection rules and permit IR-active vibrations to become Raman-visible [9].

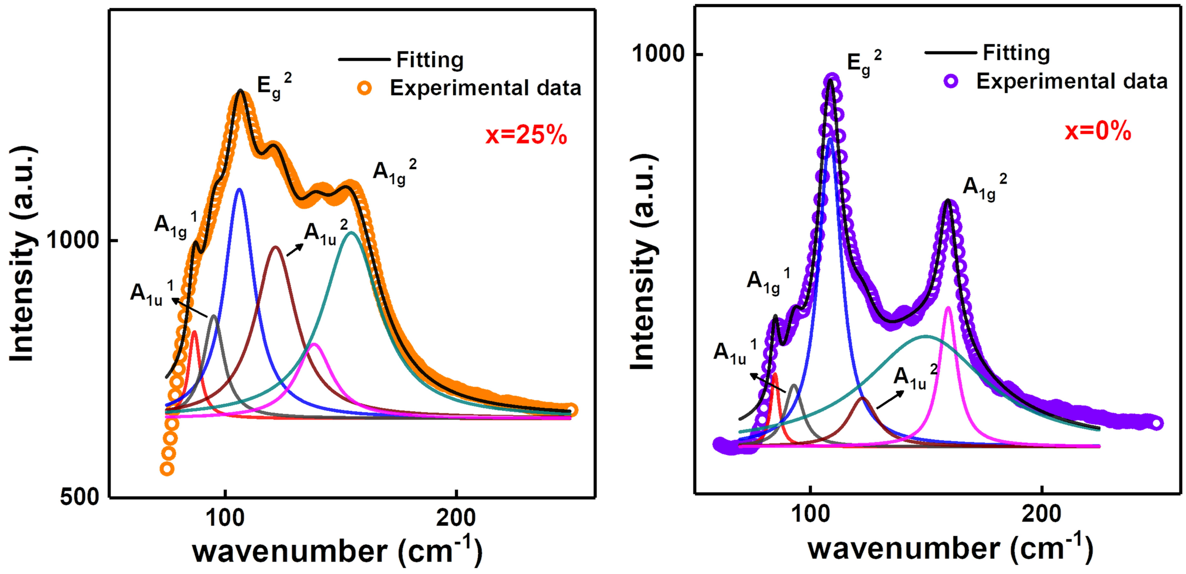


Figure 2: Raman-active and IR-active modes observed in the undoped ($x = 0\%$) and highly doped ($x = 25\%$) films. Individual vibrational features have been deconvoluted using multi-Lorentzian fitting.

With the introduction of indium into the $In_x(Bi_{0.3}Sb_{0.7})_{2-x}Te_3$ lattice, the Raman spectra undergo a noticeable evolution. The primary Raman modes broaden progressively with increasing In concentration, indicating enhanced phonon scattering arising from mass disorder and local structural distortions. Concurrently, the IR-active features become more pronounced, reflecting the gradual disruption of the long-range order of the quintuple layers. This increasing visibility of symmetry-forbidden modes, together with peak broadening, provides clear spectroscopic evidence of a systematic rise in lattice disorder as the indium content increases.

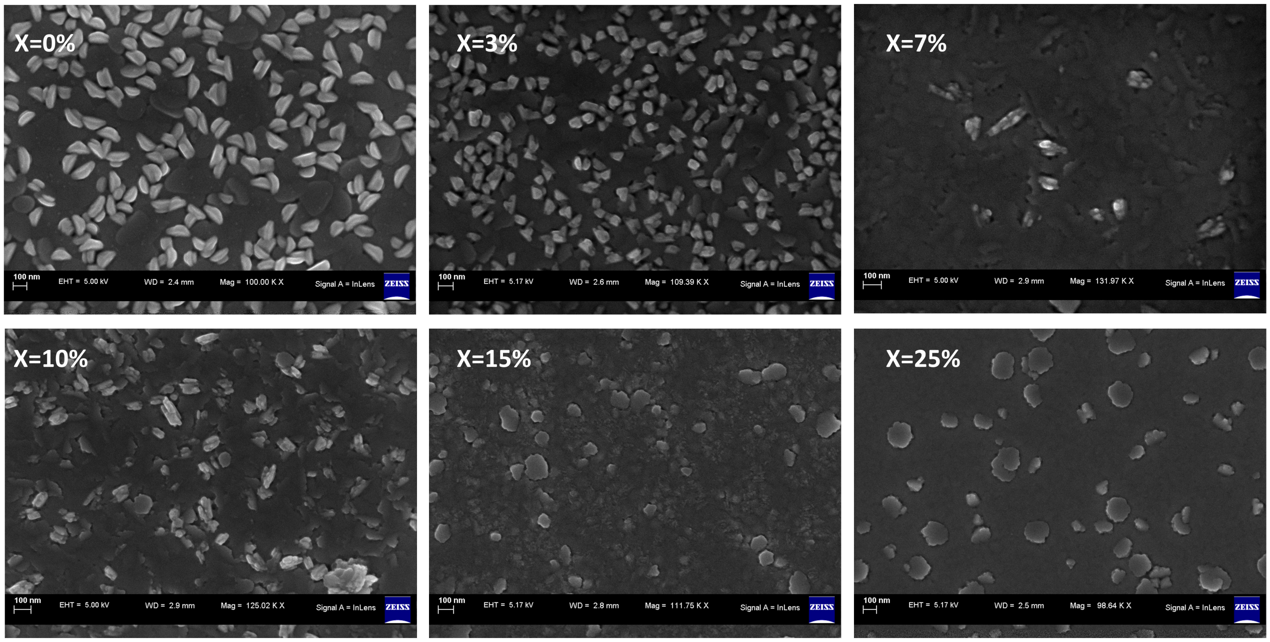


Figure 3: SEM images of $In_x(Bi_{0.3}Sb_{0.7})_{2-x}Te_3$ thin films for different indium concentrations $x$.

The SEM images show a distinct and systematic evolution in morphology with increasing indium content in the $In_x(Bi_{0.3}Sb_{0.7})_{2-x}Te_3$ films. The surface of the films displays a granular morphology, with characteristic grain sizes on the order of 100 nm. In the undoped case ($x = 0\%$), the surface is composed of well-defined, elongated rice-grain-like crystallites, which reflect anisotropic growth typical of an ordered layered structure. As indium is introduced, these features gradually lose their sharp boundaries, and the grains adopt a more rounded and diffuse appearance. This change is significant because it signals the onset of In-induced lattice disorder, which disrupts long-range crystalline uniformity. The accompanying decrease in XRD peak intensity and the increased prominence of IR-active Raman modes further support this interpretation. Thus, the observed morphological transformation provides an important microscopic signature of indium-driven disorder and its consequent influence on the electronic and transport behavior of the $In_x(Bi_{0.3}Sb_{0.7})_{2-x}Te_3$ films.

## 2: Resistance vs. Temperature analysis.

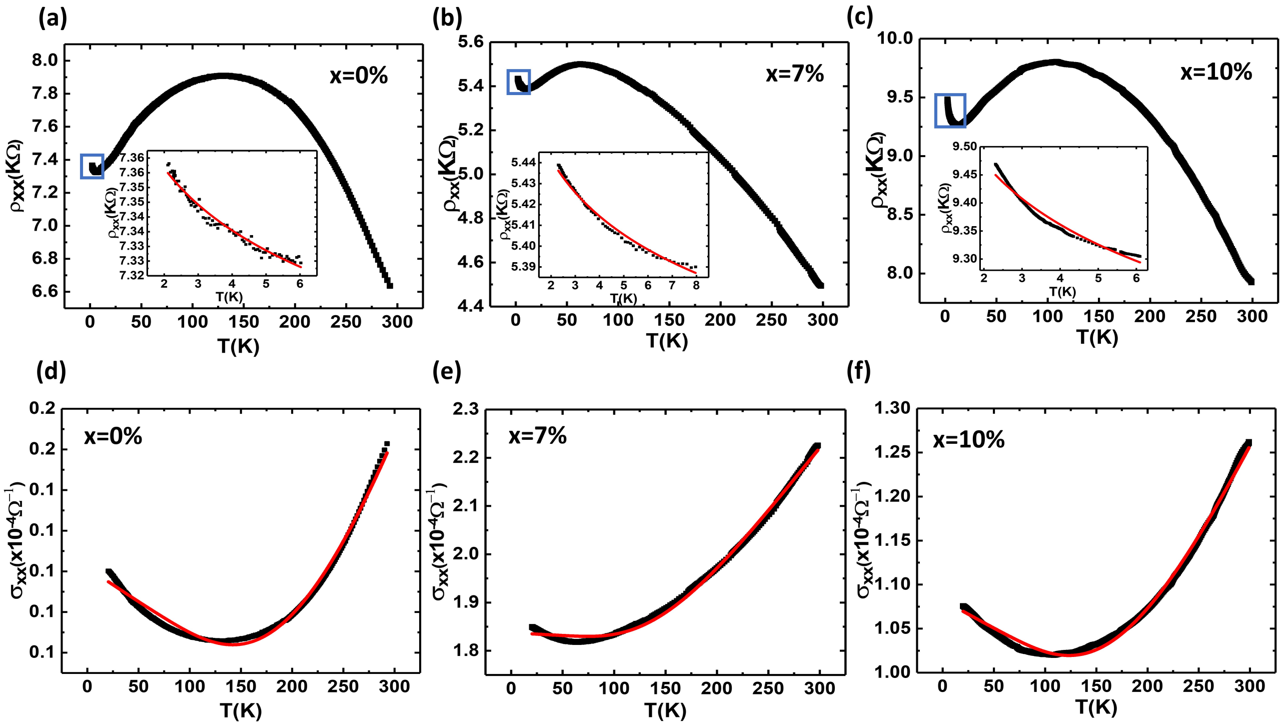


Figure 4: [a-c] Temperature dependence of the longitudinal resistance ($\rho_{xx}$) for the $\mathrm{In}_x(\mathrm{Bi}_{0.3}\mathrm{Sb}_{0.7})_{2-x}\mathrm{Te}_3$ thin film for different indium concentrations $x$. In the insets, the $\ln T$ fits are displayed as solid red lines within the low-temperature regime highlighted by the blue box. [d-f] Temperature dependence of the conductance ($\sigma_{xx}$), where the black curve represents the experimental data and the red solid line corresponds to the fit using the parallel-channel conductance model; eq(1).

For $In_x(Bi_{0.3}Sb_{0.7})_{2-x}Te_3$ thin films with composition $x < 15\%$, the temperature dependence of the conductance was analyzed using a parallel channel conductance model. In this approach, the total conductance ($\sigma_{\text{total}}$) is expressed as the sum of the bulk and surface contributions [22, 7]:

$$\begin{aligned} \sigma_{\text{total}} &= \sigma_{\text{bulk}} + \sigma_{\text{surface}} \\ &= \frac{1}{R_0\ \exp\left(\frac{\Delta}{T}\right)} + \frac{1}{A + BT}, \end{aligned} \tag{1}$$

where $\sigma_{\text{bulk}} = \dfrac{1}{R_0\ \exp(\Delta/T)}$ represents the thermally activated bulk channel with activation energy $\Delta$, and $\sigma_{\text{surface}} = \dfrac{1}{A + BT}$ describes the metallic surface channel, with $A$ accounting for disorder-induced scattering and $B$ reflecting electron–phonon interactions. At low temperatures Fig. 4(a-c), the system displays metallic characteristics, evidenced by a reduction in resistance. This trend signifies the dominance of extended, disorder-resistant surface states that continue to conduct efficiently despite scattering effects. This behavior highlights the strengthened role of surface-driven carrier transport in the low-temperature limit, a hallmark feature of topological insulators. Fig. 4(d–f) illustrates the parallel channel model fitting (solid red lines) of the conductance, and the corresponding extracted activation energies are summarized in the table.

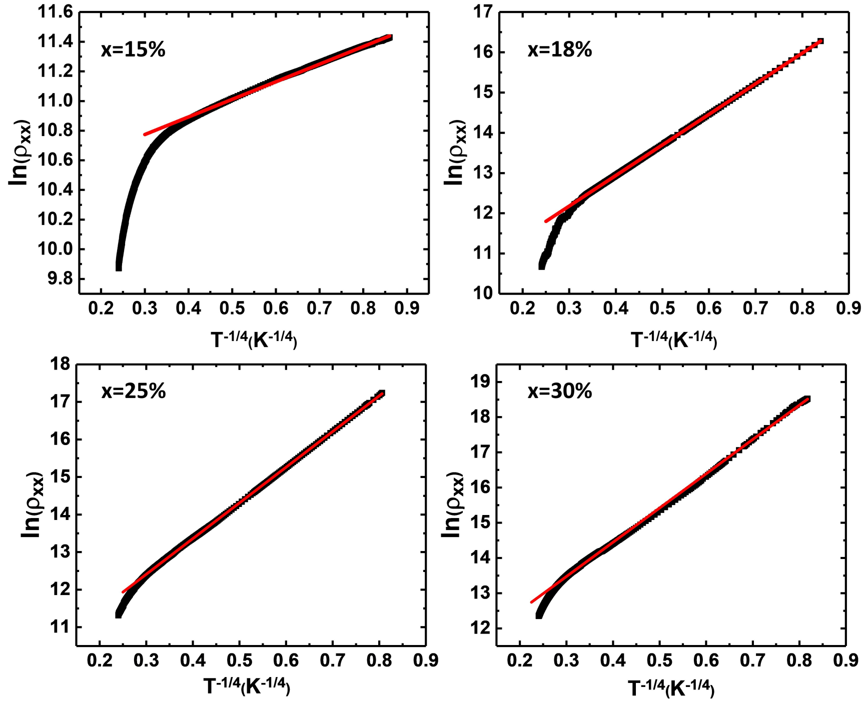


Figure 5: $\rho_{xx}$ plotted as a function of $T^{-1/4}$ for $In_x(Bi_{0.3}Sb_{0.7})_{2-x}Te_3$ samples with $x \geq 15\%$, where the solid red lines represent the Mott variable-range hopping (VRH) model fits in the low-temperature regime.

In the surface states of a topological insulator (TI), the presence of a $\pi$ Berry phase, arising from spin–momentum locking, suppresses coherent backscattering of electrons. This leads to weak antilocalization (WAL). As a result, WAL contributes a positive quantum correction to the conductivity, which increases logarithmically with decreasing temperature [6]:

$$\Delta\sigma_{\mathrm{WAL}} = \frac{e^2}{2\pi^2\hbar}\ln(T). \tag{2}$$

In contrast, electron–electron (e–e) interactions introduce a negative logarithmic correction to the conductivity, tending to reduce it at low temperatures [5]:

$$\Delta\sigma_{\text{e-e}} = -\beta\frac{e^2}{2\pi^2\hbar}\ln(T), \tag{3}$$

where $\beta$ is a material- and screening-dependent prefactor.

The total quantum correction to the surface conductivity is therefore given by the sum of these two contributions:

$$\Delta\sigma_S(T) = \Delta\sigma_{\mathrm{WAL}} + \Delta\sigma_{\text{e-e}} = \frac{e^2}{2\pi^2\hbar}\ln(T) - \beta\frac{e^2}{2\pi^2\hbar}\ln(T). \tag{4}$$

The observed low-temperature behavior of the surface conductivity in TIs is governed by the competition between WAL and e–e interaction effects, with the net logarithmic slope determined by the relative strength of these two mechanisms. We have observed that electron–electron (e–e) interactions give rise to a stronger, opposing $\ln T$ correction, which suppresses the conductivity, as illustrated in the inset of Fig. 4(a-c), $\ln(T)$ fits (solid red lines) are shown.

| x (%) | 0 | 3 | 7 | 10 | 15 |
|---|---|---|---|---|---|
| $E_A = \frac{\Delta}{K_B}(meV)$ | **71** | **68.4** | **50.6** | **59.7** | **102.2** |

Table 1: Activation energy obtained from Arrhenius fitting of the conductivity vs. temperature data for compositions with $x < 15\%$.

In samples with $x \geq 15\%$, the temperature dependence of the resistivity follows Mott's variable-range hopping (VRH) law [11]:

$$\rho(T) = \rho_0 \exp\left[\left(\frac{T_0}{T}\right)^{\frac{1}{d+1}}\right], \quad (5)$$

where $\rho(T)$ is the resistivity at temperature $T$, $\rho_0$ is a prefactor, $T_0$ is the characteristic Mott temperature, which depends on the localization length and the density of states, and $d$ denotes the dimensionality of the system (2, or 3). The low-temperature transport behavior is well described by three-dimensional Mott variable-range hopping (VRH), and the characteristic parameters $T_0$ were obtained from the fitting. The temperature range over which Mott VRH remains valid increases systematically with $x$. Specifically, the VRH regime extends up to approximately 50 K, 70 K, 85 K, 110 K, and 150 K for $x = 15\%, 18\%, 20\%, 25\%$, and 30%, respectively. At higher temperatures beyond these limits, the resistivity deviates from the VRH description and follows a thermally activated behavior. The extracted $T_0$ values of 2.03, 480, 2531, 4430, and 9432 are consistent with the energy scales expected for variable-range hopping (VRH) transport, indicating that conduction in this regime is governed by localized states. For the highest substitution level ($x = 30\%$), the obtained $T_0$ remains within the VRH framework but suggests that the hopping mechanism is approaching its limit of validity. This observation is consistent with earlier reports on the topological-metal to band-insulator transition in $(Bi_{1-x}In_x)_2Se_3$ thin films [3].

## 3: Magnetoconductance Analysis.

Magnetoconductivity (MC), defined as $\Delta\sigma = \sigma(B) - \sigma(0)$, exhibits distinct behavior depending on disorder. For films in the diffusive regime, the negative MC can be described using the Hikami–Larkin–Nagaoka (HLN) model [8, 4]:

$$\Delta\sigma(B) = -\alpha\frac{e^2}{2\pi^2\hbar}\left[\psi\left(\frac{1}{2}+\frac{B_\phi}{B}\right) - \ln\left(\frac{B_\phi}{B}\right)\right] + \beta B^2 \tag{6}$$

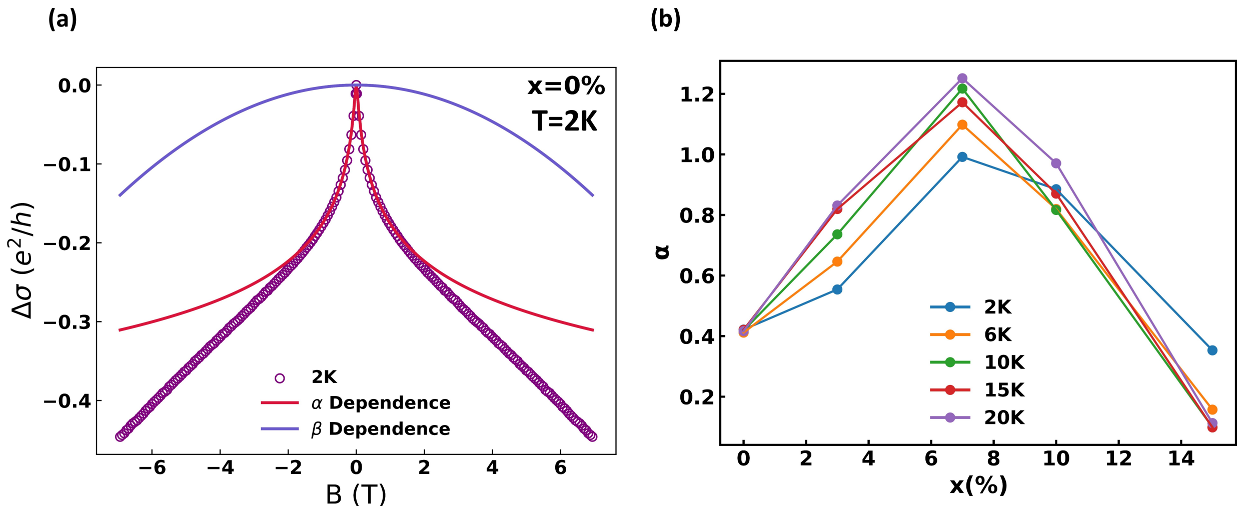


Figure 6: (a) Magnetoconductance of the thin film with $x = 0\%$. The Hikami–Larkin–Nagaoka (HLN) prefactor $\alpha$ and the quadratic background coefficient $\beta$ extracted from the fitting are plotted separately. (b) Temperature dependence of the HLN prefactor $\alpha$ for different doping concentrations $x$, obtained from analysis of the weak antilocalization magnetoconductance.

Here, $\psi$ is the digamma function, and $B_\phi = \hbar/(4el_\phi^2)$ is the dephasing field related to the phase coherence length $l_\phi$. The prefactor $\alpha$ indicates the effective number of two-dimensional conduction channels, with an ideal value of 1 for topological insulator (TI) thin films where the top and bottom surface states contribute independently (each contributing 1/2). The coefficient $\beta$ accounts for classical cyclotronic effects as well as elastic and spin-orbit scattering contributions [1].

### 3.1: Behavior of the WAL Fitting Parameter $\alpha$

In the Hikami–Larkin–Nagaoka (HLN) description of weak antilocalization, the fitting parameter $\alpha$ reflects the effective number of independent, phase-coherent two-dimensional transport channels that contribute to quantum interference. A value of $\alpha \approx 0.5$ is generally associated with a single symplectic channel, such as one topological surface state. When both the top and bottom surfaces of a thin film participate independently, $\alpha$ approaches 1. Values of $\alpha$ exceeding 1 in magnitude are sometimes reported and are typically attributed to contributions from multiple electronic subbands, the presence of trivial two-dimensional electron gases, or complex coupling between parallel conduction channels [18, 2].

When indium is introduced into $In_x(Bi_{0.3}Sb_{0.7})_{2-x}Te_3$, several electronic and structural modifications arise before the system reaches the critical concentration at which band inversion collapses. At low In content, substitution primarily introduces disorder and perturbs the bulk electronic

structure without destroying the inverted band gap. This disorder suppresses bulk conduction by disrupting impurity-band–mediated transport and by altering the effective bulk gap, thereby enhancing the surface contribution to charge transport. As the bulk channel becomes increasingly insulating, the top and bottom surface states lose their mutual coupling and begin to act as independent phase-coherent channels[5, 13]. Consequently, the Hikami–Larkin–Nagaoka prefactor $\alpha$ evolves from its single-channel value of approximately 0.5 toward 1, reflecting two decoupled spin-momentum–locked Dirac channels. Additional disorder-induced suppression of interband scattering between Dirac bands and trivial bulk subbands further sharpens the weak antilocalization (WAL) response, contributing to the enhancement of $\alpha$.

This trend is fully consistent with the observed increase of the WAL prefactor from $\alpha = 1/2$ to $\alpha = 1$ as the indium concentration rises from 0% to 7%. The evolution reflects a transition from effectively one to two topological surface transport channels, facilitated by the defect-state engineering role of indium identified by Sharma *et al.* [17]. In the undoped limit, residual bulk defects and impurity bands promote inter-channel scattering between the top and bottom surfaces, reducing the number of independent quantum conduction channels. With increasing In content, the suppression of shallow impurity states and the reconfiguration of deep antisite defects[17] enhance the bulk insulating character and strongly diminish this coupling. As a result, both surfaces contribute independently to the WAL effect, yielding the full theoretical prefactor of $\alpha = 1$.

The microscopic origin of this evolution is closely related to the orbital character of the electronic states. In the parent compound $(Bi_{0.3}Sb_{0.7})_2Te_3$, the conduction band is primarily composed of Bi/Sb 6$p$ orbitals, while the valence band is dominated by Te 5$p$ orbitals. Strong spin-orbit coupling inverts these bands, stabilizing the topological insulating phase with gapless Dirac surface states. With indium substitution, the In 5$s$ orbitals strongly hybridize with Te 5$p$ states, modifying the band ordering and progressively weakening the inverted 6$p$-band character. This hybridization reduces bulk conduction while preserving the topological surface states in the pre-transition regime [10, 24], which explains the increase in $\alpha$. As the indium concentration approaches the critical value, the In 5$s$ states dominate the conduction band, the inverted band structure collapses, and the topological surface states disappear. Consequently, weak antilocalization is suppressed, and $\alpha$ decreases.

### 3.2: Phase coherence length vs. Temperature.

The phase coherence length, representing the characteristic length scale over which charge carriers preserve quantum phase coherence, is determined from the Hikami–Larkin–Nagaoka (HLN) weak antilocalization fitting. With increasing disorder, the extracted exponent $\gamma$ in the relation $l_\phi \propto T^{-\gamma}$ decreases from approximately 0.5 toward values much smaller than 1. The initial value, $\gamma \approx 0.5$, is consistent with the expected 2D diffusive regime where electron–electron interactions dominate phase decoherence. As disorder increases, the exponent gradually reduces to $\sim 0.38$–0.36, indicating a departure from simple 2D diffusive behavior. This reduction may arise from a combination of effects, including a dimensional crossover to percolating transport channels [20], a suppression of the effective diffusion constant with disorder, or the emergence of additional dephasing mechanisms such as inelastic scattering from localized states. At stronger disorder, the exponent drops to very small values ($\sim 0.15$), reflecting a transition to a transport regime dominated by strong localization and variable-range hopping (VRH). In this regime, the diffusive phase-coherence picture underlying the Hikami–Larkin–Nagaoka (HLN) model becomes inapplicable, and the extracted $l_\phi$ represents an effective length rather than a true phase coher-

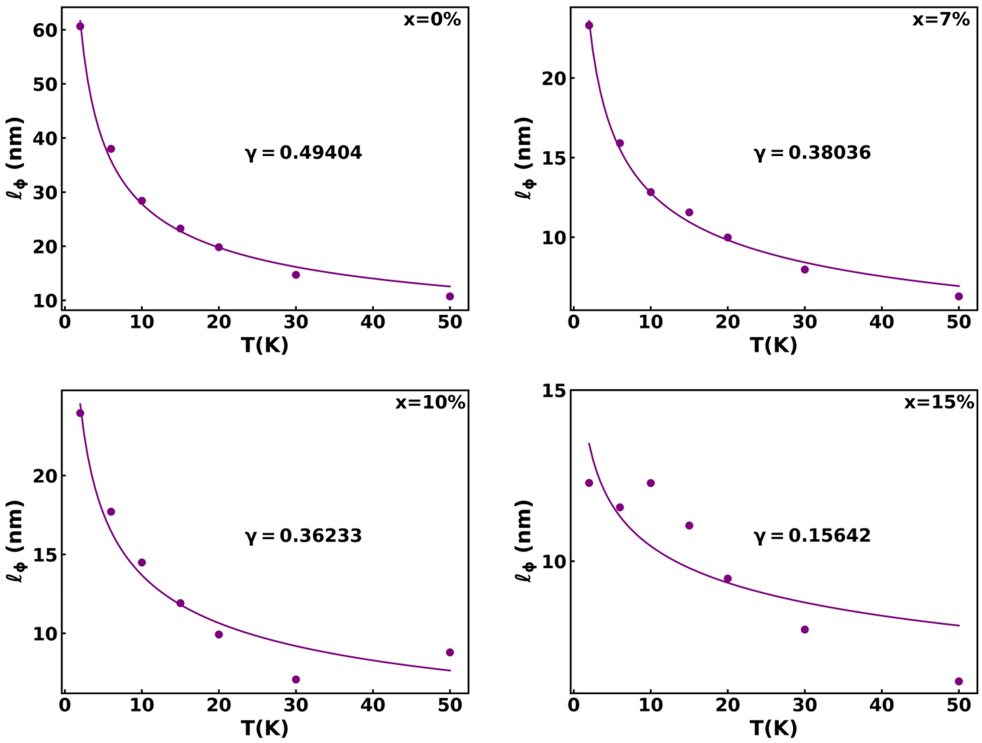


Figure 7: Phase coherence length vs. temperature for $In_x(Bi_{0.3}Sb_{0.7})_{2-x}Te_3$ thin films with $x$ as 0%, 7%, 10% and 15%. The variation with temperature is fitted with the power law $l_\phi \propto T^{-\gamma}$ (solid line).

ence length. Such a trend highlights the crossover from diffusive electron transport to hopping between localized states, where coherence is limited by tunneling processes rather than conventional diffusive dephasing. This interpretation is supported by the observed VRH temperature dependence of the conductivity, the reduction of the HLN fitting parameter $\alpha$, and the evolution of the magnetoconductance shape

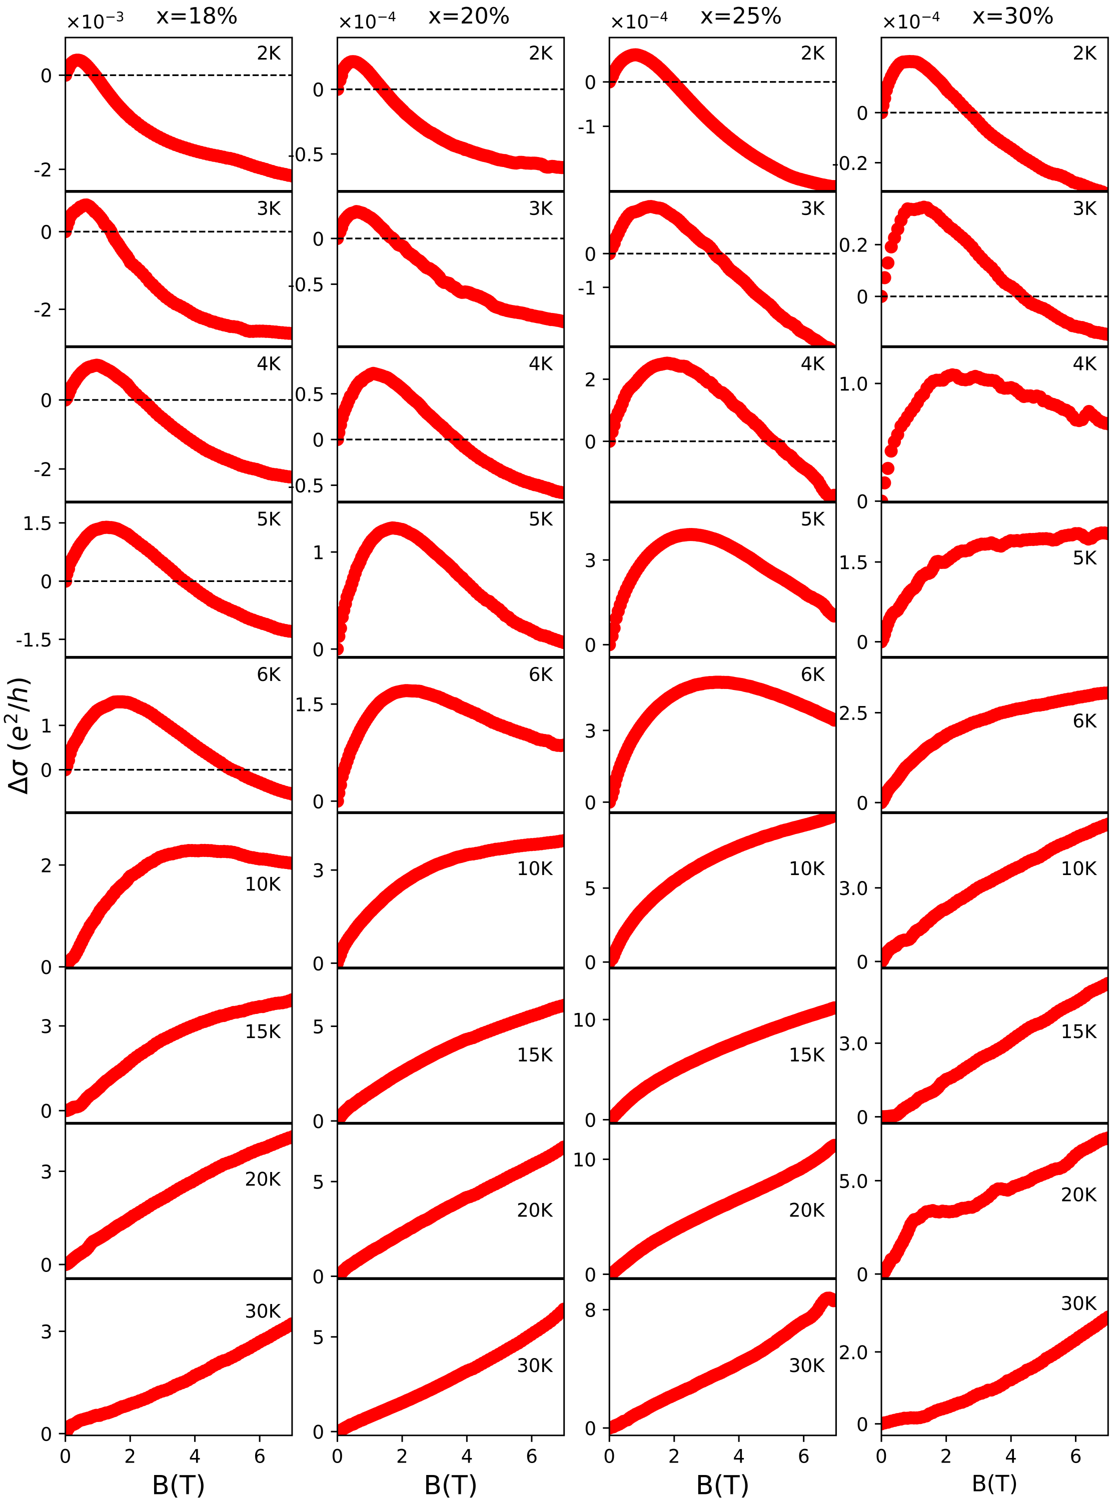


Figure 8: Representative magnetoconductance curves for various temperatures and doping levels $x$, illustrating the systematic evolution of the magnetoconductive response with both temperature and impurity concentration.

## 4: Magnetic-Field Effects and Wave-Function Shrinkage in Mott Variable-Range Hopping regime.

In disordered systems exhibiting Mott variable-range hopping (VRH), the zero-field resistivity is described by the Mott law [11]:

$$\rho(T) = \rho_0 \exp\left[\left(\frac{T_0}{T}\right)^{1/(d+1)}\right], \tag{7}$$

where $d$ is the system dimensionality ($d = 2$ or 3), $\rho_0$ is a prefactor, and

$$T_0 = \frac{\beta}{k_B N(E_F)\xi^d}. \tag{8}$$

Here, $N(E_F)$ is the microscopic single-particle density of states at the Fermi level, $\xi$ is the localization length, $k_B$ is the Boltzmann constant, and $\beta$ is a numerical constant determined by percolation theory [19]. The typical hopping distance $r_{\text{opt}}$ and energy window $\varepsilon_{\text{opt}}$ are obtained from the percolation condition, which requires that the number of accessible states within a hopping volume of radius $r$ and energy width $\varepsilon$ satisfies

$$r^d N(E_F)\varepsilon \sim 1. \tag{9}$$

From this, the optimal hopping parameters are

$$r_{\text{opt}} \sim \xi\left(\frac{T_0}{T}\right)^{1/(d+1)}, \quad \varepsilon_{\text{opt}} \sim k_B T\left(\frac{T_0}{T}\right)^{1/(d+1)}. \tag{10}$$

When a perpendicular magnetic field $B$ is applied, the decay of localized wavefunctions acquires a Gaussian factor due to orbital shrinkage:

$$\psi(r, B) \sim \psi(r, 0)\exp\left[-\frac{r^2}{4l_B^2}\right], \tag{11}$$

where $l_B = \sqrt{\hbar/(eB)}$ is the magnetic length, $\hbar$ is the reduced Planck constant, and $e$ is the elementary charge. The corresponding tunneling probability between two sites separated by distance $r$ becomes

$$W(r; B) \propto \exp\left[-\frac{2r}{\xi} - \frac{r^2}{4l_B^2}\right]. \tag{12}$$

The first term represents the exponential decay of the wavefunction over distance $\xi$, while the second term accounts for the suppression of long-range hops by the magnetic field. To satisfy the percolation condition in the presence of $B$, the reduced hopping distance $r_{\text{opt}}(B) < r_{\text{opt}}(0)$ is compensated by an increased energy window $\varepsilon_{\text{opt}}(B)$, ensuring

$$r_{\text{opt}}^d N(E_F)\varepsilon_{\text{opt}} \sim 1. \tag{13}$$

Consequently, the number of states available for transport effectively increases. This is captured by defining an effective density of states

$$N_{\text{eff}}(E_F, B) \approx N(E_F)H(B, T), \tag{14}$$

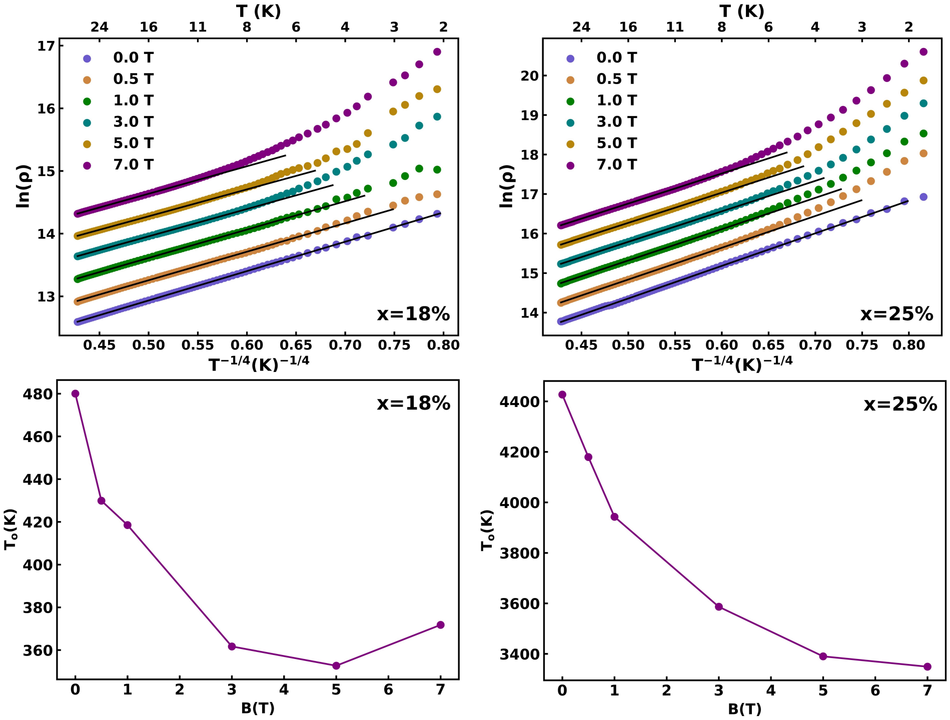


Figure 9: Temperature-dependent resistivity of $In_x(Bi_{0.3}Sb_{0.7})_{2-x}Te_3$ samples with $x \geq 15\%$ measured under various magnetic fields. The linear dependence of $\ln\rho$ on $T^{-1/4}$ confirms Mott three-dimensional variable–range hopping within the VRH regime, from which the characteristic temperature $T_0$ is obtained. A systematic decrease in $T_0$ with increasing magnetic field is observed.

where $H(B,T) > 1$ is a dimensionless factor describing the enhancement of transport-relevant states due to wave-function shrinkage [14, 15].The apparent decrease in $T_0$ in finite-field fits reflects the effective DOS enhancement $H(B,T)$, not a true change in microscopic parameters [14, 15, 19].

In samples with $x \geq 15\%$, the temperature-dependent resistivity was measured under various applied magnetic fields, as shown in the figure. At very low temperatures, the data exhibit deviations from the zero-field 3D Mott variable–range hopping (VRH) behavior; however, within the temperature range where VRH remains the dominant conduction mechanism, the Mott relation is still satisfied. This is confirmed by the linear dependence of $\ln\rho$ on $T^{-1/4}$, from which the characteristic Mott temperature $T_0$ is extracted. A systematic decrease in $T_0$ is observed with increasing magnetic field. This reduction does not indicate a genuine modification of the microscopic localization length or the intrinsic density of states, but instead reflects the magnetic-field-induced enhancement of the effective density of states accessible for hopping transport, consistent with the wave-function–shrinkage mechanism proposed by Raikh et.al.

## 4.1: Low field regime

At very low temperatures and small magnetic fields, hopping transport can also exhibit a negative magnetoresistance linear in $B$, arising from quantum interference between multiple hopping paths, as described by Nguyen, Spivak, and Shklovskii (NSS) [12] and observed in $\delta$-doped GaAs layers [23]. The tunneling amplitude between sites $i$ and $j$ is

$$\mathcal{A}_{ij} = \sum_p \mathcal{A}_p, \quad \mathcal{A}_p \sim e^{-r_p/\xi} e^{i\phi_p}, \tag{15}$$

where $r_p$ is the path length and $\phi_p$ is the phase accumulated along the path. In zero magnetic field, each path has a time-reversed counterpart $-p$, and destructive interference reduces the hopping probability. A small magnetic field introduces an Aharonov-Bohm phase

$$\phi_B = \frac{e}{\hbar} \int_p \mathbf{A} \cdot d\mathbf{l}, \tag{16}$$

where $\mathbf{A}$ is the vector potential, and the integral is taken along the hopping path $p$ with line element $d\mathbf{l}$; breaking time-reversal symmetry and enhancing the hopping probability. In this regime, the relative resistivity change is linear:

$$\frac{\Delta\rho(B)}{\rho(0)} \sim -\frac{B}{B_c}, \tag{17}$$

with

$$B_c \sim \frac{\hbar}{e r_{\text{hop}}^2}, \quad r_{\text{hop}}(T) \sim \xi \left(\frac{T_0}{T}\right)^{1/(d+1)}, \tag{18}$$

where $r_{\text{hop}}$ is the typical hopping distance at temperature $T$. The slope of this negative linear MR decreases with increasing temperature. This effect persists only for $B \ll B_c$, beyond which the positive quadratic MR from orbital shrinkage dominates. Dimensionality affects the magnitude and crossover field, but the qualitative mechanism is the same. Therefore, in Mott VRH, the overall magnetoresistance combines a low-field negative linear MR due to quantum interference (NSS) and a high-field positive quadratic MR from wave-function shrinkage and enhanced effective DOS as proposed by Raikh et.al.

# References


[1] Badih A Assaf et al. “Linear magnetoresistance in topological insulator thin films: Quantum phase coherence effects at high temperatures”. In: *Applied Physics Letters* 102.1 (2013).

[2] Lihong Bao et al. “Weak anti-localization and quantum oscillations of surface states in topological insulator Bi2Se2Te”. In: *Scientific reports* 2.1 (2012), p. 726.

[3] Matthew Brahlek et al. “Topological-metal to band-insulator transition in (Bi 1-x In x) 2 Se 3 thin films”. In: *Physical review letters* 109.18 (2012), p. 186403.

[4] Matthew Brahlek et al. “Transport properties of topological insulators: Band bending, bulk metal-to-insulator transition, and weak anti-localization”. In: *Solid State Communications* 215 (2015), pp. 54–62.

[5] Shao-Pin Chiu and Juhn-Jong Lin. “Weak antilocalization in topological insulator Bi 2 Te 3 microflakes”. In: *Physical Review B—Condensed Matter and Materials Physics* 87.3 (2013), p. 035122.

[6] Ion Garate and Leonid Glazman. “Weak localization and antilocalization in topological insulator thin films with coherent bulk-surface coupling”. In: *Physical Review B—Condensed Matter and Materials Physics* 86.3 (2012), p. 035422.

[7] Radha Krishna Gopal et al. “Topological delocalization and tuning of surface channel separation in Bi2Se2Te Topological Insulator Thin films”. In: *Scientific Reports* 7.1 (2017), p. 4924.

[8] Shinobu Hikami, Anatoly I Larkin, and Yosuke Nagaoka. “Spin-orbit interaction and magnetoresistance in the two dimensional random system”. In: *Progress of Theoretical Physics* 63.2 (1980), pp. 707–710.

[9] Fengjiao Liu et al. “A micro-Raman study of exfoliated few-layered n-type Bi2 Te2. 7Se0. 3”. In: *Scientific reports* 7.1 (2017), p. 16535.

[10] Jianpeng Liu and David Vanderbilt. “Topological phase transitions in (Bi 1- x In x) 2 Se 3 and (Bi 1- x Sb x) 2 Se 3”. In: *Physical Review B—Condensed Matter and Materials Physics* 88.22 (2013), p. 224202.

[11] Nevill Francis Mott and Edward A Davis. *Electronic processes in non-crystalline materials.* OUP Oxford, 2012.

[12] VL Nguen, BZ Spivak, and BI Shkovskii. “Tunnel hopping in disordered systems”. In: *Zh. Eksp. Teor. Fiz* 89 (1985), p. 1770.

[13] Hanbum Park et al. “Disorder-induced decoupled surface transport channels in thin films of doped topological insulators”. In: *Physical Review B* 98.4 (2018), p. 045411.

[14] ME Raikh. “Incoherent mechanism of negative magnetoresistance in the variable-range-hopping regime”. In: *Solid state communications* 75.11 (1990), pp. 935–938.

[15] ME Raikh et al. “Mechanisms of magnetoresistance in variable-range-hopping transport for two-dimensional electron systems”. In: *Physical Review B* 45.11 (1992), p. 6015.

[16] Zhi Ren et al. “Optimizing Bi 2-x Sb x Te 3-y Se y solid solutions to approach the intrinsic topological insulator regime”. In: *Physical Review B—Condensed Matter and Materials Physics* 84.16 (2011), p. 165311.

[17] Kanav Sharma et al. "Suppression of Generation-Recombination Noise in Topological Insulators Through Indium Substitution". In: *arXiv preprint arXiv:2410.06291* (2024).

[18] Chandra Shekhar et al. "Evidence of surface transport and weak antilocalization in a single crystal of the Bi 2 Te 2 Se topological insulator". In: *Physical Review B* 90.16 (2014), p. 165140.

[19] Boris Isaakovich Shklovskii and Alex L Efros. *Electronic properties of doped semiconductors*. Vol. 45. Springer Science & Business Media, 2013.

[20] Brian Skinner, Tianran Chen, and BI Shklovskii. "Why is the bulk resistivity of topological insulators so small?" In: *Physical review letters* 109.17 (2012), p. 176801.

[21] Chunxiao Wang et al. "In situ Raman spectroscopy of topological insulator Bi2Te3 films with varying thickness". In: *Nano Research* 6.9 (2013), pp. 688–692.

[22] Yang Xu et al. "Observation of topological surface state quantum Hall effect in an intrinsic three-dimensional topological insulator". In: *Nature Physics* 10.12 (2014), pp. 956–963.

[23] Qiu-yi Ye et al. "Hopping transport in $\delta$-doping layers in GaAs". In: *Physical Review B* 41.12 (1990), p. 8477.

[24] Zhen-Yu Ye et al. "The origin of electronic band structure anomaly in topological crystalline insulator group-IV tellurides". In: *npj Computational Materials* 1.1 (2015), pp. 1–6.

[25] Chaohua Zhang et al. "Controlled growth of bismuth antimony telluride BixSb2- xTe3 nanoplatelets and their bulk thermoelectric nanocomposites". In: *Nano Energy* 15 (2015), pp. 688–696.
